# Supplementary material for: Band-Mott mixing hybridizes the gap in Fe$_2$Mo$_3$O$_8$
Source: arXiv:2203.02402 source file (2022-03-04)
Supplement: Supplementary file 1 [file Supplementary_information_for_Band_Mott_mixing_hybridizes_the_gap_in_Fe2Mo3O8.pdf]

# Supplementary Information for “Band-Mott mixing hybridizes the gap in $\text{Fe}_2\text{Mo}_3\text{O}_8$ ”

K. Park,<sup>1,2</sup> G. L. Pascut,<sup>1,3</sup> G. Khanal,<sup>4</sup> M. O. Yokosuk,<sup>2</sup> Xianghan Xu,<sup>4</sup> Bin Gao,<sup>5</sup> M. J. Gutmann,<sup>6</sup> A. P. Litvinchuk,<sup>7</sup> V. Kiryukhin,<sup>4,8</sup> S. -W. Cheong,<sup>4,8,9</sup> D. Vanderbilt,<sup>4</sup> K. Haule,<sup>4</sup> and J. L. Musfeldt<sup>2,10</sup>

<sup>1</sup>*These authors contributed equally to this work*

<sup>2</sup>*Department of Chemistry, University of Tennessee, Knoxville, Tennessee 37996, USA*

<sup>3</sup>*MANSiD Research Center and Faculty of Forestry,  
Applied Ecology Laboratory, Stefan Cel Mare University (USV),  
13 University Rd, Suceava 720229, Romania*

<sup>4</sup>*Department of Physics and Astronomy,  
Rutgers University, Piscataway, New Jersey 08854, USA*

<sup>5</sup>*Department of Physics and Astronomy,  
Rice University, Houston, Texas 77005, USA*

<sup>6</sup>*ISIS Facility, STFC-Rutherford Appleton Laboratory,  
Didcot OX11 0QX, United Kingdom*

<sup>7</sup>*Texas Center for Superconductivity and Department of Physics,  
University of Houston, Houston, Texas 77204, USA*

<sup>8</sup>*Rutgers Center for Emergent Materials,  
Rutgers University, Piscataway, New Jersey 08854, USA*

<sup>9</sup>*Laboratory for Pohang Emergent Materials and Max  
Planck POSTECH Center for Complex Phase Materials,  
Pohang University of Science and Technology, Pohang 790-784, Korea*

<sup>10</sup>*Department of Physics and Astronomy,  
University of Tennessee, Knoxville, Tennessee 37996, USA*

(Dated: October 28, 2021)

### Local $C_{3v}$ symmetry splits the $d$ orbitals in $\text{Fe}_2\text{Mo}_3\text{O}_8$

Figure S1 summarizes the local symmetry of the trigonally-distorted octahedral and tetrahedral sites in  $\text{Fe}_2\text{Mo}_3\text{O}_8$ . These labels are used extensively in the main text and also here in Supplementary Information.

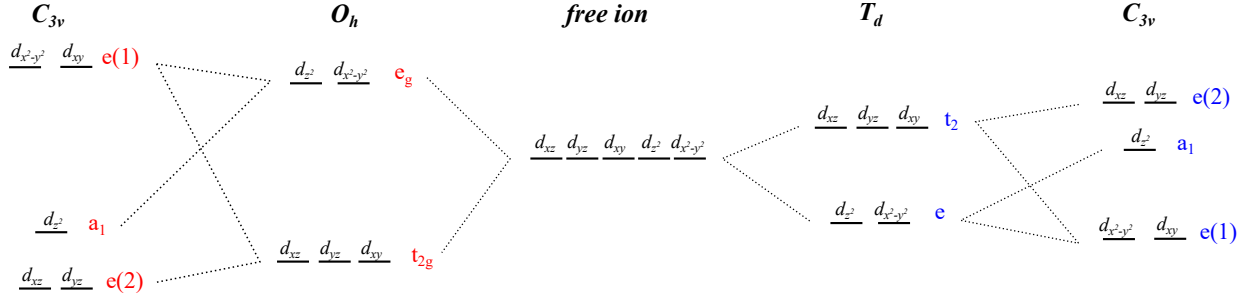

FIG. S1. Diagram of  $d$ -orbital splitting from free ion states to octahedral + tetrahedral symmetries to  $C_{3v}$  local symmetry for the distorted octahedral and tetrahedral sites in  $\text{Fe}_2\text{Mo}_3\text{O}_8$ . States of  $e$  and  $a_1$  symmetry are revealed in both the trigonally-distorted octahedra and tetrahedra. For clarity, we label the degenerate  $d_{x^2-y^2}$  and  $d_{xy}$  set of orbitals as  $e(1)$  whereas the doubly degenerate  $d_{xz}$  and  $d_{yz}$  set are labeled as  $e(2)$ . The  $d_{z^2}$  orbital always transforms as  $a_1$ . Note that the order of the  $e$  symmetry orbitals is swapped on the distorted octahedral and tetrahedral sites, and the  $a_1$  symmetry orbital is always associated with the  $e(2)$  pair.

### Optical properties of $\text{Ni}_2\text{Mo}_3\text{O}_8$ and $\text{Mn}_2\text{Mo}_3\text{O}_8$

In order to explore structure-property relationships in the  $A_2\text{Mo}_3\text{O}_8$  family of materials, we measured a number of Zn-substituted analogs of  $\text{Fe}_2\text{Mo}_3\text{O}_8$  as well as  $\text{Ni}_2\text{Mo}_3\text{O}_8$  and  $\text{Mn}_2\text{Mo}_3\text{O}_8$ . Figure S2(a,b) displays the linear absorption spectra of  $\text{Ni}_2\text{Mo}_3\text{O}_8$  and  $\text{Mn}_2\text{Mo}_3\text{O}_8$ . The Ni compound sports a complicated set of  $d$ -to- $d$  excitations near 0.25, 0.6, 1.1, and 1.5 eV whereas the Mn system has only one  $d$ -to- $d$  excitation centered near 1 eV. In both cases, the  $d$ -to- $d$  excitations reside inside the gap. We extracted the charge gaps of  $\text{Ni}_2\text{Mo}_3\text{O}_8$  and  $\text{Mn}_2\text{Mo}_3\text{O}_8$  with plots of  $(\alpha \cdot E)^2$  vs. energy and find that they are very similar to that in  $\text{Zn}_2\text{Mo}_3\text{O}_8$ . This comparison shows that chemical bonding in  $\text{Fe}_2\text{Mo}_3\text{O}_8$  is special and merits further investigation.

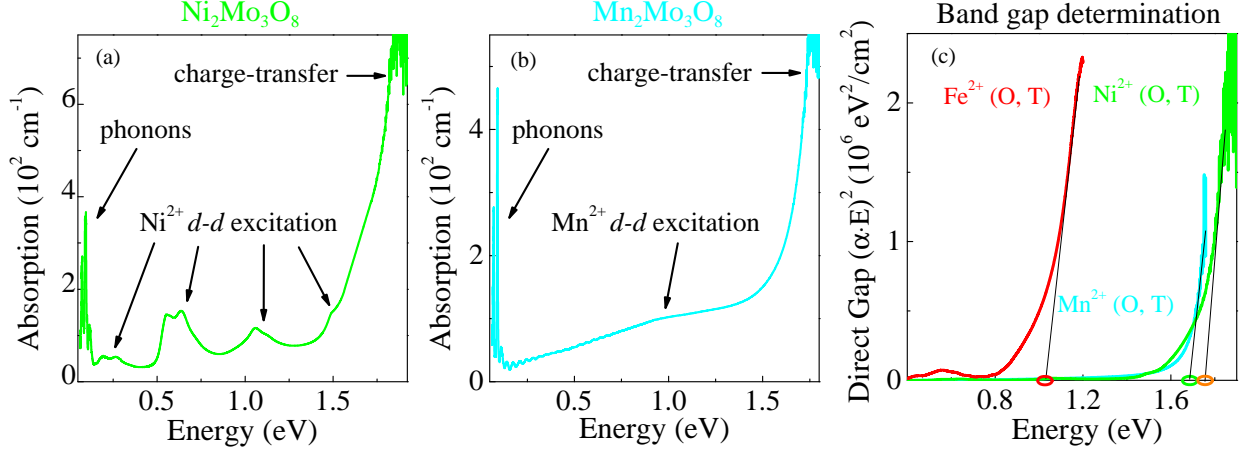

FIG. S2. (a,b) Absorption spectra of  $\text{Ni}_2\text{Mo}_3\text{O}_8$  and  $\text{Mn}_2\text{Mo}_3\text{O}_8$  single crystals in the  $ab$ -plane at room temperature. (c) A Tauc plot is used to extract the direct band gap of these materials.

### Optical properties of $\text{FeZnMo}_3\text{O}_8$ as a function of temperature

The optical properties of  $\text{FeZnMo}_3\text{O}_8$  are summarized in Fig. S3. This system has Zn in the T site leaving  $\text{Fe}^{2+}$  in the O site. The  $\text{Fe}(\text{O})$  site excitation appears near 1 eV - the same energy as in  $\text{Fe}_2\text{Mo}_3\text{O}_8$ , but with slightly more separation between the local excitation and charge transfer band. The temperature dependence of this structure is shown in Fig. S3(f), and changes in the oscillator strength with temperature can be quantified with a modified vibronic coupling model. This is just like  $\text{Fe}_2\text{Mo}_3\text{O}_8$ , albeit with a somewhat lower coupling phonon frequency. The temperature dependence of the band gap in  $\text{FeZnMo}_3\text{O}_8$  is fairly linear, different from that in the two end members [Fig. S3(b,c)].

Crystal quality played an especially important role in our measurements of  $\text{FeZnMo}_3\text{O}_8$ . The sequence of our work compared to that of other groups was also to our advantage. The authors of Refs. [S1, S2] had already done the majority of their work by the time we started ours, so the crystal growth team enjoyed more time to improve sample growth protocols. As a result, we measured higher quality materials with very well-controlled Zn substitution. At the same time, we benefited from a comparison with the spectroscopic findings in Refs. [S1, S2]. Although our work doesn't focus on vibrational properties, this comparison identified a number of issues, and we refined our methods based upon what we learned. Two factors differentiate our crystals from those in Refs. [S1, S2]: well-controlled crystal stoichiometry and optical density. Stoichiometric  $\text{FeZnMo}_3\text{O}_8$  single crystals obviously enabled unambiguous assignment and analysis of the  $d$ -to- $d$  on-site excitations. This is different from

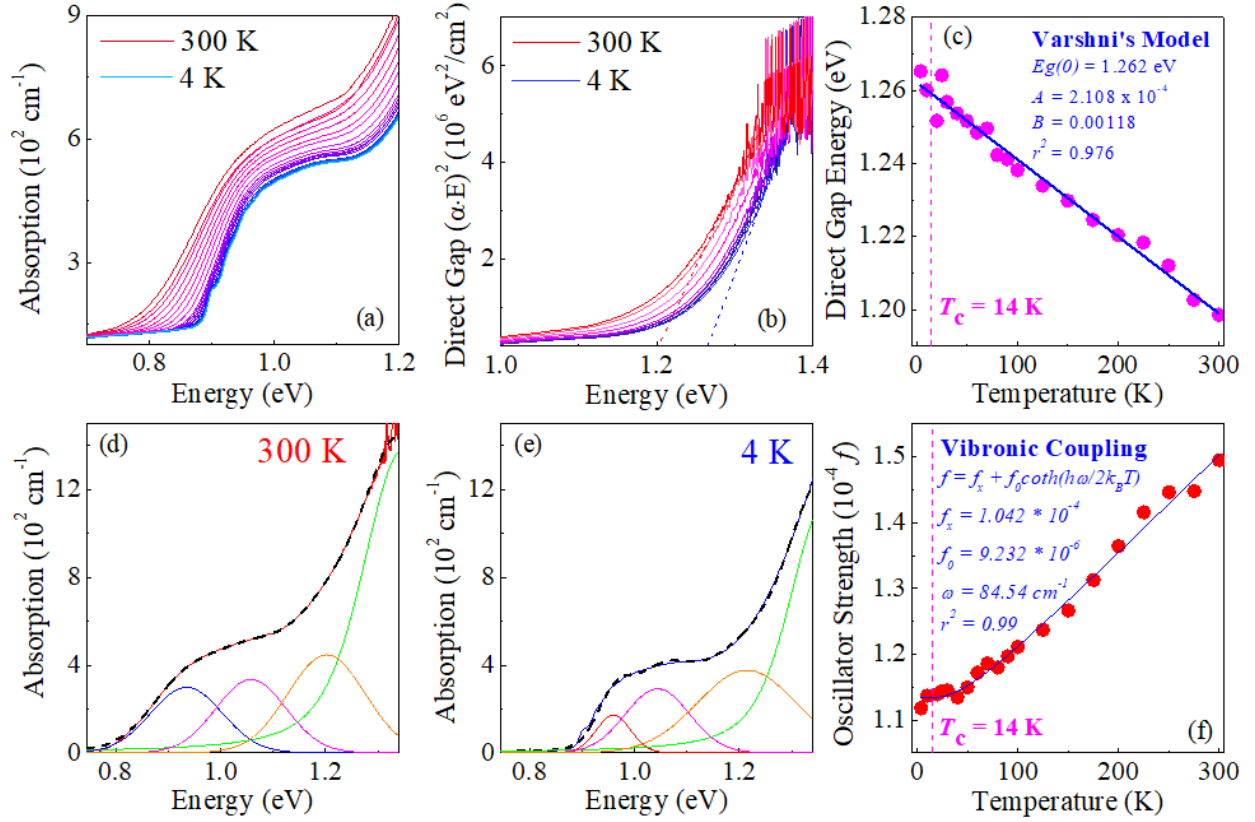

FIG. S3. (a) Linear absorption spectra of FeZnMo<sub>3</sub>O<sub>8</sub> as function of temperature. (b) Tauc plot to extrapolate the band gap. (c) Direct gap energy vs. temperature and fit to the Varshni model. (d,e) Peak fit of the Fe<sup>2+</sup> *d*-to-*d* excitation on the Fe(O) site at 300 K and 4 K, respectively. (f) Oscillator strength vs. temperature and fit to a modified vibronic coupling model.

Ref. [S1], where the reflectance spectra shows some sample dependence - especially in the vicinity of the tetrahedral Fe *d*-to-*d* band near 0.5 eV. The latter depends crucially on Fe (and Zn) concentration. This took some time and many repeated measurements with different crystals to unravel, but with proper samples, the trends are very logical. The authors of Ref. [S1] also see light leakage. If a sample is too thin, a reflectance measurement will have problems because instead of reflecting, light can transmit through the sample - at least at certain energies. It is therefore important that the sample be thick enough to avoid this problem. Unfortunately, crystals in this family of materials do not naturally grow very thick. With temperature, the Fe<sub>2</sub>Mo<sub>3</sub>O<sub>8</sub> family of materials expand and contract, which changes the degree of leakage as well. The prior authors commented about this fact in their paper. We encountered this problem early on just like they did, which is why we decided to per-

form transmittance experiments. This obviates the light leakage problem entirely but makes certain optical constants inaccessible.

### Band gap vs. temperature for the $A_2\text{Mo}_3\text{O}_8$ materials ( $A = \text{Fe, Zn, Ni and Mn}$ )

Figure S4(a-d) shows Tauc plots for several different  $A_2\text{Mo}_3\text{O}_8$  analogs in order to illustrate how the direct band gaps are determined. Figure S4(e-h) show how the gap changes with temperature as well as fits to the Varshni model [S3, S4]. The latter is a semi-empirical model evaluating nonlinear behavior of the charge gap vs. temperature. It is expressed as:  $E_g(T) = E_g(0) - \frac{AT^2}{T+B}$ , where  $E_g(0)$  is the limiting low temperature value of the band gap,  $T$  is temperature, and  $A$  and  $B$  are fit parameters. As mentioned in the main text, the band gap of  $\text{Fe}_2\text{Mo}_3\text{O}_8$  drops across the 61 K magnetic ordering transition - deviating from the Varshni model fit. The band gaps of the analogs shown here are not sensitive to their respective magnetic ordering transitions. The Zn, Mn, and Ni analogs have a standard curvature whereas  $\text{FeZnMo}_3\text{O}_8$  has a surprisingly linear trend. The parameters for the Varshni model fits are shown in Table S1.

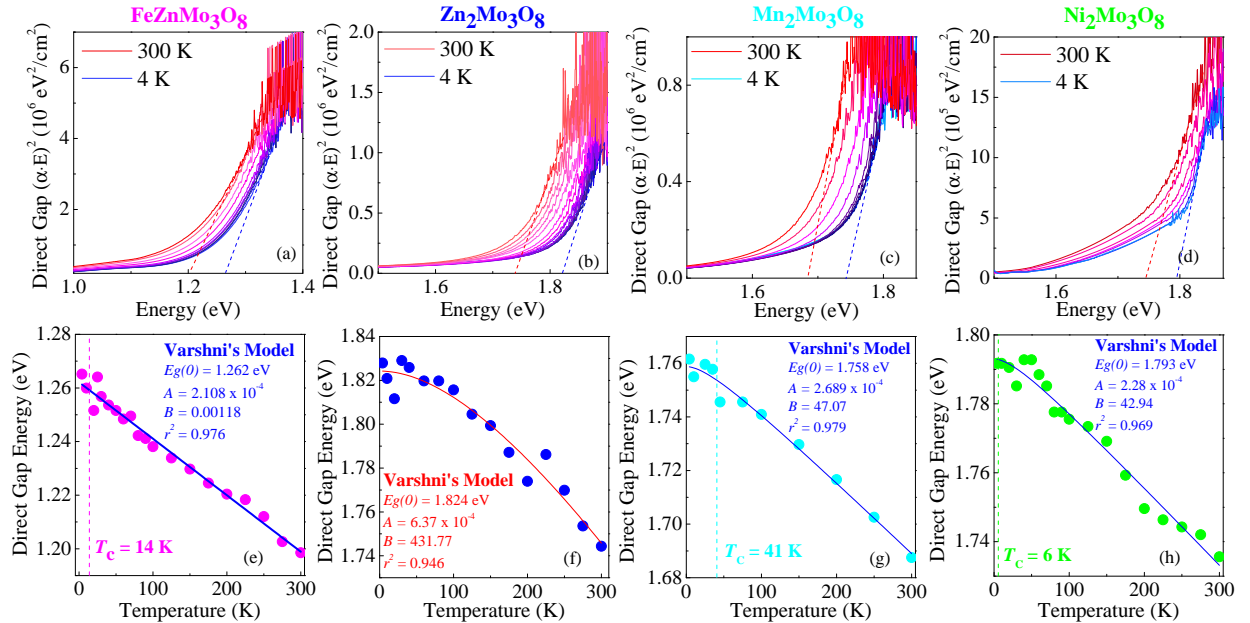

FIG. S4. (a-d) Plots of  $(\alpha \cdot E)^2$  vs. energy are used to reveal direct band gap energies via extrapolation for the  $\text{FeZnMo}_3\text{O}_8$ ,  $\text{Zn}_2\text{Mo}_3\text{O}_8$ ,  $\text{Mn}_2\text{Mo}_3\text{O}_8$ , and  $\text{Ni}_2\text{Mo}_3\text{O}_8$  materials. (e-h) Band gap vs. temperature for each of these compounds along with fits to the Varshni model.

TABLE S1. Summary of Varshni model fit parameters for the temperature dependence of the band gap for  $\text{Fe}_2\text{Mo}_3\text{O}_8$  and the other analogs of interest in this work.

| Material                           | $A$                   | $B$   | $E_g(0)$ (eV) | $r^2$ |
|------------------------------------|-----------------------|-------|---------------|-------|
| $\text{Fe}_2\text{Mo}_3\text{O}_8$ | $6.57 \times 10^{-4}$ | 705.7 | 1.08          | 0.96  |
| $\text{FeZnMo}_3\text{O}_8$        | $2.11 \times 10^{-4}$ | 0.001 | 1.26          | 0.98  |
| $\text{Zn}_2\text{Mo}_3\text{O}_8$ | $6.37 \times 10^{-4}$ | 431.8 | 1.82          | 0.95  |
| $\text{Mn}_2\text{Mo}_3\text{O}_8$ | $2.69 \times 10^{-4}$ | 47.07 | 1.76          | 0.98  |
| $\text{Ni}_2\text{Mo}_3\text{O}_8$ | $2.28 \times 10^{-4}$ | 42.94 | 1.79          | 0.97  |

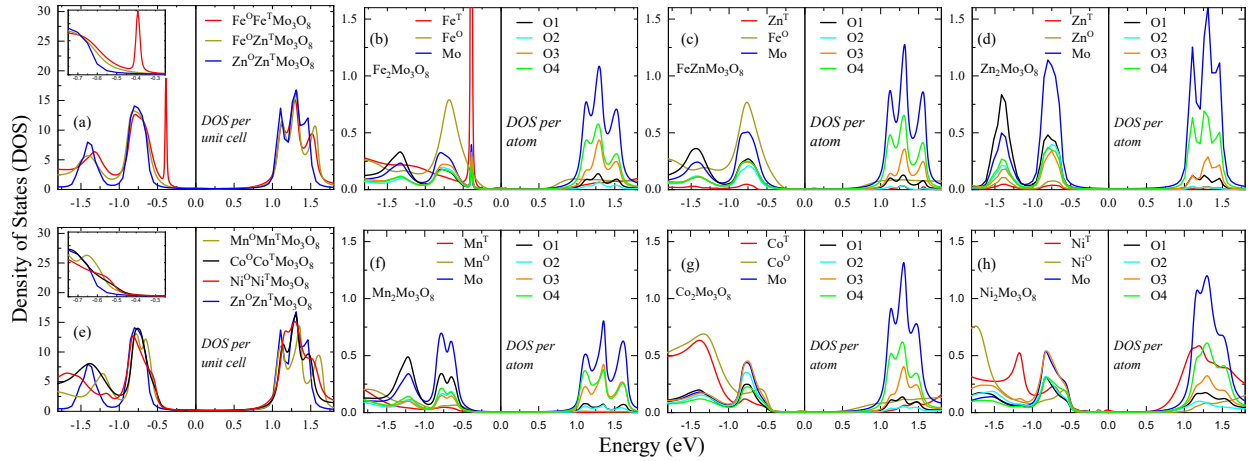

FIG. S5. Density of states for the materials of interest in this work. Panels (a) and (e) show the density of states per unit cell. Panels (b-d) and (f-h) show the density of states per A, Mo, and O atom. Only  $\text{Fe}_2\text{Mo}_3\text{O}_8$  has the strong, sharp resonance near the Fermi energy.

### Unit cell and atom projected density of states

Figure S5 summarizes the electronic density of states projected per unit cell and per atom for the  $A_2\text{Mo}_3\text{O}_8$  compounds where  $A = \text{Mn}, \text{Fe}, \text{Co}, \text{Ni}$  and  $\text{Zn}$ , respectively.

### Spectral functions, self-energies, and orbital density of states

Figures S5 - S9 show the spectral functions, orbital projected density of states, and the self-energies corresponding to the orbitals of the different materials in question. The nature of the Mott gap is proved by the existence of a pole in the self-energy within the gap. The nature of the band gap is demonstrated by the absence of a self-energy pole within the gap.

The self-energy on the real axis was obtained using the analytical continuation maximum entropy method for the local cumulant as explained in [S21].

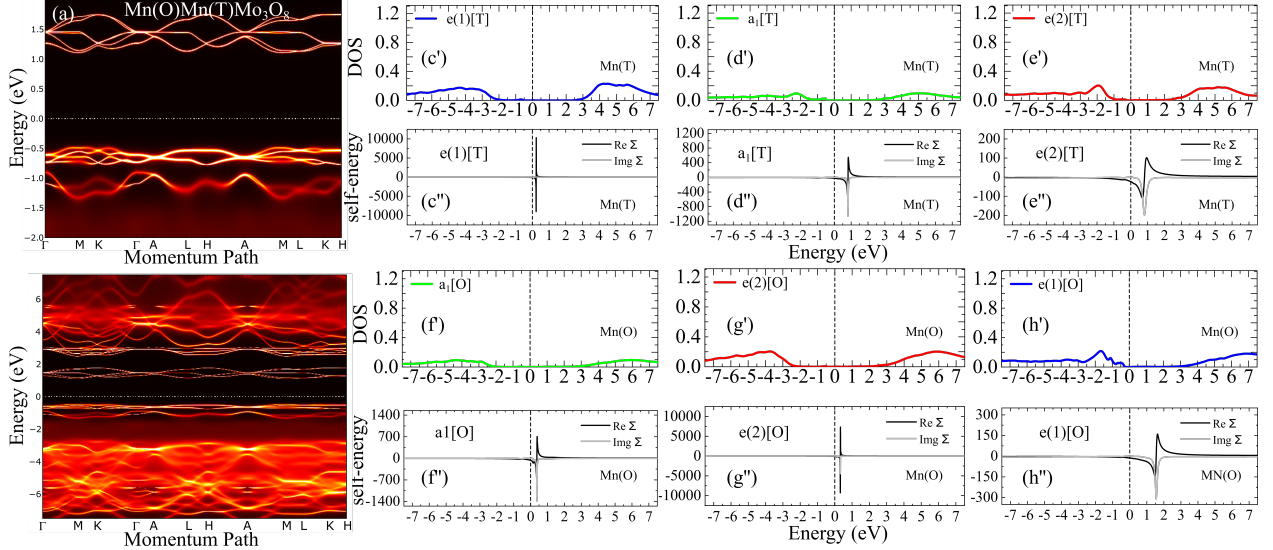

FIG. S6.  $\text{Mn}_2\text{Mo}_3\text{O}_8$ : Panels (a) and (b) show the spectral functions for two different energy ranges; Panel (c) to (h) show the orbital projected density of states together with the real and imaginary self-energies for the corresponding orbital. The panels labelled by the prime symbols correspond to the orbital projected density of states, and those labelled by double prime correspond to the self-energies.

### On-site excitations in the $A_2\text{Mo}_3\text{O}_8$ ( $A = \text{Fe}, \text{Zn}$ ) family of materials

There are several additional aspects to the electronic structure of  $\text{Fe}_2\text{Mo}_3\text{O}_8$  including the two on-site  $d$ -to- $d$  excitations centered near 0.5 and 0.95 eV, respectively. Focusing first on the  $d$ -to- $d$  excitation emanating from the distorted octahedral  $\text{Fe}^{2+}$  site [Fig. S11(c)], we see that it strongly overlaps with the charge gap excitation. To separate these effects, we fit the  $d$ -to- $d$  excitations with three oscillators plus the gap edge. The sum of these three peaks provides the oscillator strength of the on-site excitation [Fig. S11(f)]. We quantified the temperature dependence of the oscillator strength with a modified vibronic coupling model as  $f = f_x + f_0 \coth(h \frac{\omega}{2k_B T})$  [S6–S9]. Here,  $f_0$  is the oscillator strength at base temperature,  $f_x$  is the oscillator strength from other mixing processes,  $\omega$  is the frequency of the activating phonon,  $h$  is Planck's constant,  $k_B$  is the Boltzmann constant, and  $T$  is the temperature. The overall quality of the fit in Fig. S11(f) is typical, and we extract a coupling phonon

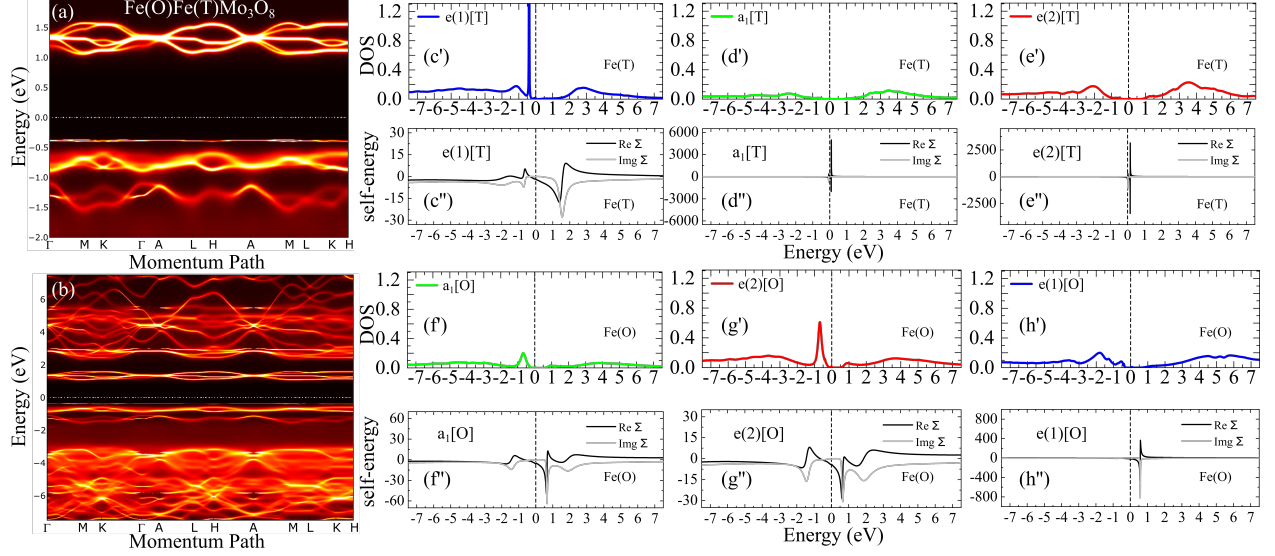

FIG. S7.  $\text{Fe}_2\text{Mo}_3\text{O}_8$ : Panels (a, b) show the spectral functions for two different energy ranges; Panels (c-h) show the orbital projected density of states along with the real and imaginary self-energies for the corresponding orbital. The panels labelled by prime symbols correspond to orbital projected density of states, and those labelled as double prime correspond to self-energies.

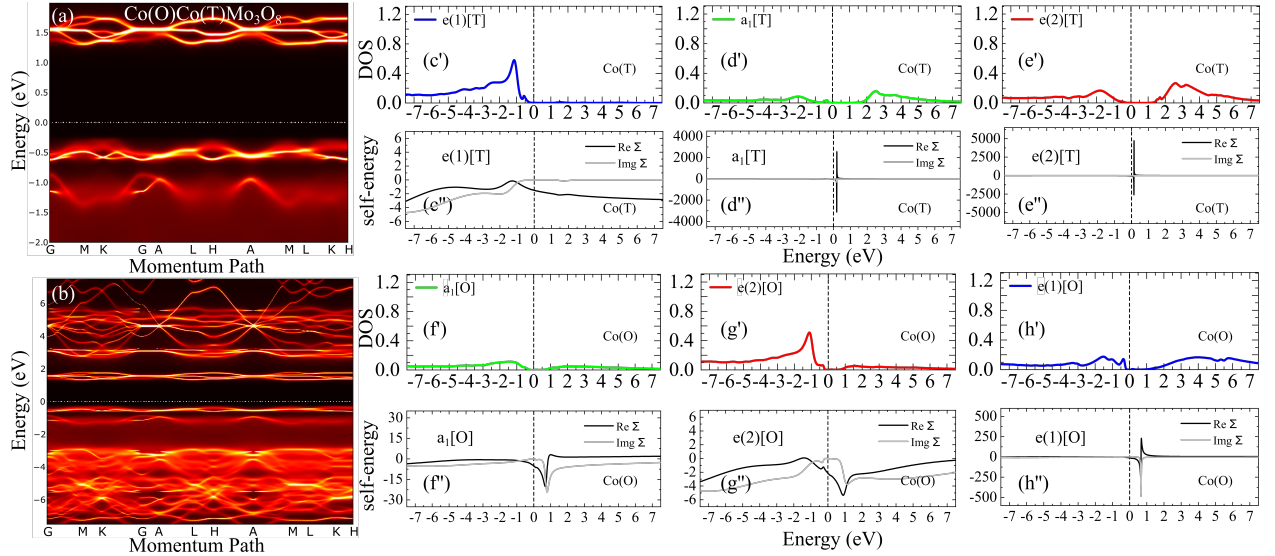

FIG. S8.  $\text{Co}_2\text{Mo}_3\text{O}_8$ : Panels (a) and (b) show the spectral functions for two different energy ranges; Panel (c) to (h) show the orbital projected density of states together with the real and imaginary self-energies for the corresponding orbital. The panels labelled by the prime symbols correspond to the orbital projected density of states, and those labelled by double prime correspond to the self-energies.

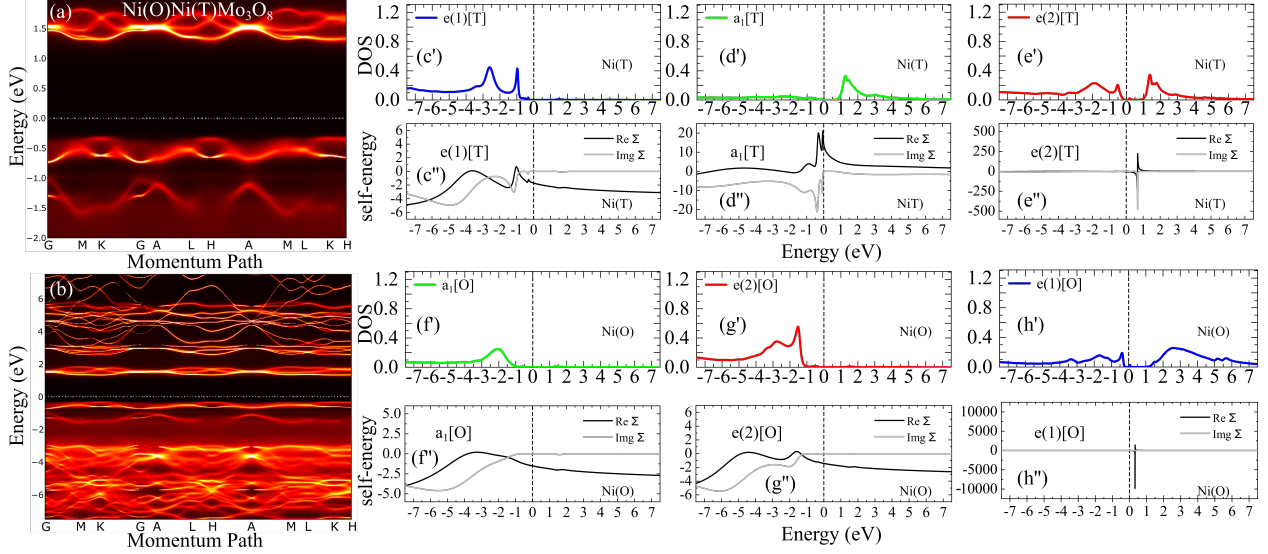

FIG. S9.  $\text{Ni}_2\text{Mo}_3\text{O}_8$ : Panels (a) and (b) show the spectral functions for two different energy ranges; Panel (c) to (h) show the orbital projected density of states together with the real and imaginary self-energies for the corresponding orbital. The panels labelled by the prime symbols correspond to the orbital projected density of states, and those labelled by double prime correspond to the self-energies.

frequency of  $151 \text{ cm}^{-1}$ . This value is in excellent agreement with the  $E_1$  symmetry phonon at  $144 \text{ cm}^{-1}$  reported by Stanislavchuk *et. al.* [S1] and Reschke *et. al.* [S2]. Examination of the displacement pattern of this mode reveals a complex combination of Fe(T) distortion + twisting of the Mo trimer + stretching one of the edge-sharing O centers between  $\text{FeO}_6$  and the Mo trimer [Fig. S12]. This distinct oxygen involvement modulates the Mo-O-Fe angle and thus the Mo trimer  $\cdots$  Fe(O) interaction. Examination of the local crystal structure [S2, S5] reveals that the  $\text{FeO}_6$  is trigonally distorted, so coupling with an odd-symmetry infrared-active phonon is required to activate this  $d$ -to- $d$  excitation. We also carried out a vibronic coupling analysis of the  $d$ -to- $d$  on-site excitation in  $\text{FeZnMo}_3\text{O}_8$ . Vibronic coupling activates the octahedral Fe site excitation in this system as well [Fig. S3(f)].

Next we turn our attention to the  $d$ -to- $d$  excitation near 0.5 eV that emanates from the  $\text{Fe}^{2+}$  center in the tetrahedral environment. What differentiates this on-site excitation from that on the octahedral site is the dramatic fine structure that develops below the magnetic ordering transition [Fig. S11(b)]. A similar response is observed in  $\text{Fe}^{2+}:\text{ZnSe}$  [S10]. Here, the  $\text{Fe}^{2+}$  ions are well isolated in the ZnSe matrix, and they sport a distorted tetrahedral

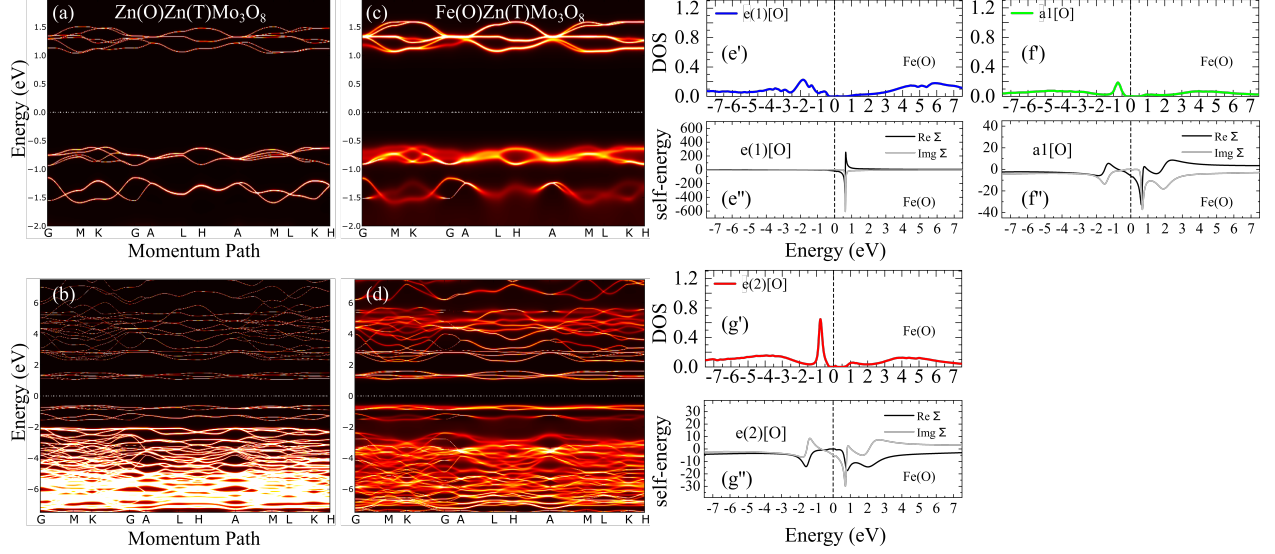

FIG. S10.  $\text{Zn}_2\text{Mo}_3\text{O}_8$  and  $\text{FeZnMo}_3\text{O}_8$ : Panel (a) to (d) show the spectral functions for two different energy range; Panels (e) to (g) show the orbital projected density of states together with the real and imaginary self-energies for the corresponding orbital. The panels labelled by the prime symbols correspond to the orbital projected density of states, and those labelled by double prime correspond to the self-energies.

crystal field - just like  $\text{Fe}_2\text{Mo}_3\text{O}_8$ . The activation mechanism for the fine structure includes a combination of crystal field effects, spin-orbit coupling, and dynamic Jahn-Teller distortion [S10]. Overall, the low temperature spectrum of  $\text{Fe}_2\text{Mo}_3\text{O}_8$  is in remarkable agreement with that of  $\text{Fe}^{2+}:\text{ZnSe}$  in terms of peak positions, intensities, and the detailed splitting pattern [S10] suggesting that the mechanism is identical. We also carried out an oscillator strength analysis [Fig. S11(e)]. Despite the dramatic appearance of the aforementioned fine structure, the oscillator strength of the  $\text{Fe}^{2+}$   $d$ -to- $d$  excitation on the distorted tetrahedral site is conserved as a function of temperature. Elongation of the  $\text{FeO}_4$  tetrahedron appears to obviate the need for vibronic coupling while, at the same time, providing a mechanism for the development of polarization [S11].

### Vibronic coupling and the displacement pattern of the $E_1$ symmetry mode

As discussed in the prior section, the  $\text{Fe}^{2+}$  on-site  $d$ -to- $d$  excitation on the trigonally-distorted octahedral site is activated by a modified vibronic coupling [S6–S9]. One characteristic of this model is the odd-symmetry coupling phonon. A fit of the vibronic model to our data

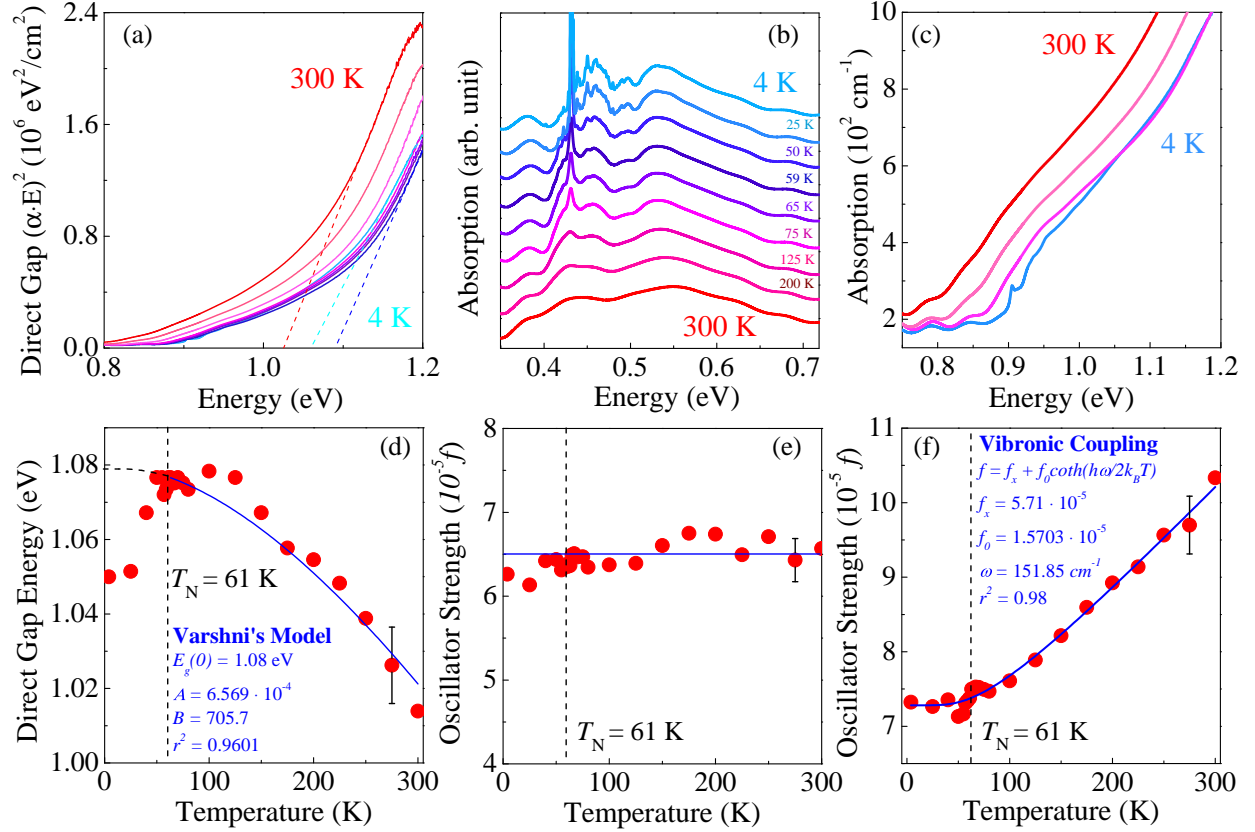

FIG. S11. (a, d) Tauc plot of  $(\alpha \cdot E)^2$  vs. energy for  $\text{Fe}_2\text{Mo}_3\text{O}_8$  and a plot of band gap vs. temperature with a fit to the Varshni model. (b, e) Close-up view of the  $\text{Fe}^{2+}$   $d$ -to- $d$  on-site excitation on the distorted tetrahedral site showing the fine structure that develops due to spin-orbit coupling below the 61 K magnetic ordering transition. (c, f) Close-up view of the  $\text{Fe}^{2+}$   $d$ -to- $d$  on-site excitation on the distorted octahedral site and oscillator strength vs. temperature along with a fit to the vibronic coupling model [S6].

yields a coupled phonon frequency of  $151 \text{ cm}^{-1}$  in excellent agreement with the  $E_1$  symmetry vibrational mode at  $144 \text{ cm}^{-1}$  [S1, S2]. The displacement pattern of this highly collective mode is shown in Fig. S12. It is quite complex. One oxygen is distorting the quasi-octahedral environment via the displacement of Mo trimer. The Fe(T) center displaces as well, but it does not have any affect on the octahedral site. It is the modulation of the  $\text{Fe}(\text{O}) \cdots \text{O} \cdots \text{Mo}$  connection that matters here. The  $\text{Fe}^{2+}$   $d$ -to- $d$  excitation on the trigonally-distorted tetrahedral site is not activated by vibronic coupling.

FIG. S12. Schematic view of the displacement pattern of the  $144\text{ cm}^{-1}$   $E_1$  symmetry vibrational mode. As discussed in the main text, this odd-symmetry mode is responsible for vibronically activating the  $\text{Fe}^{2+}$   $d$ -to- $d$  transition on the trigonally-distorted octahedral site in  $\text{Fe}_2\text{Mo}_3\text{O}_8$ .

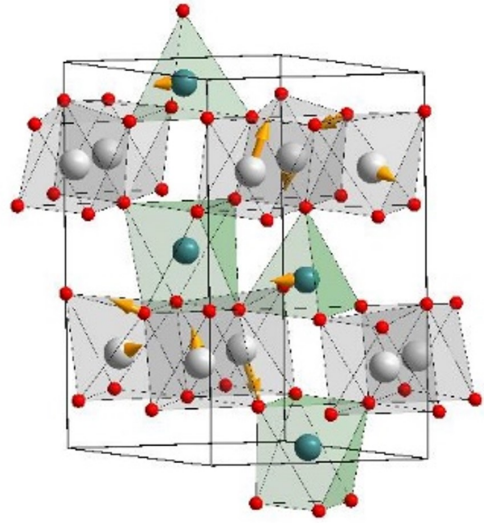

### Fitting the $d$ -to- $d$ excitations of $\text{Fe}_2\text{Mo}_3\text{O}_8$

We employed Voigt oscillators to fit the  $\text{Fe}^{2+}$   $d$ -to- $d$  excitations in  $\text{Fe}_2\text{Mo}_3\text{O}_8$ . Figure S13 shows examples of fits to the on-site excitations at 300 and 4.2 K. Here, three Voigt oscillators are employed to model the excitation on the  $\text{Fe}(\text{O})$  site, and an additional peak is used to account for the edge of the charge transfer band. This separation of local electronic excitations gives a better understanding of changes in the  $\text{Fe}(\text{O})$  excitations as a function of temperature. We note in passing that the small sharp feature near 0.9 eV may be a magnon sideband. Measurements in a magnetic field will help clarify this assignment. For the  $\text{Fe}(\text{T})$  site excitations in Fig. S13 (c,d), nine peaks are used for the fit although not all of the oscillators are physically meaningful due to the low temperature fine structure.

### Crystal structures for $A_2\text{Mo}_3\text{O}_8$ ( $A = \text{Mn}, \text{Fe}, \text{Co}, \text{Ni}, \text{Zn}$ )

A Rigaku Oxford Diffraction SuperNova diffractometer equipped with an Atlas CCD-detector and Cu K- $\alpha$  radiation was used to perform single crystal diffraction measurements. Data collected at  $T = 300\text{ K}$  were analyzed (cell refinement and reduction) by CRYSTALISPRO software [S12]. The structure refinement was performed by JANA2006 software [S13]. Other technical details such as absorption and extinction corrections were discussed previously [S1, S14, S15]. Images of the crystal structures were generated using the VESTA software [S16]. Other images were prepared using INKSCAPE [S17]. The coordinates for each of the materials in this series are summarized in the Tables below.

FIG. S13. (a,b) Example peak fits using Voigt oscillators for the  $\text{Fe}^{2+}$   $d$ -to- $d$  excitation on the Fe(O) site in  $\text{Fe}_2\text{Mo}_3\text{O}_8$  at 300 and 4 K, respectively. (c,d) Peak fits for the  $\text{Fe}^{2+}$   $d$ -to- $d$  excitation on the Fe(T) site in  $\text{Fe}_2\text{Mo}_3\text{O}_8$  at 300 and 4 K, respectively.

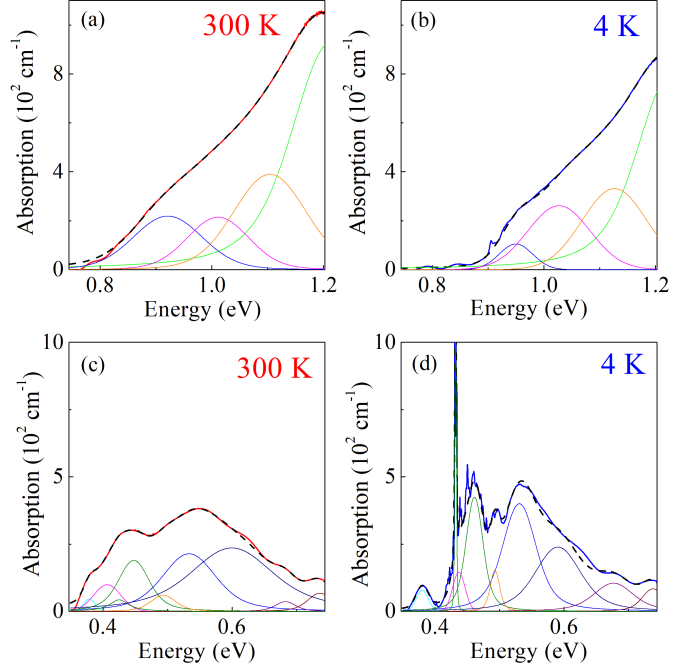

TABLE S2.  $\text{Ni}_2\text{Mo}_3\text{O}_8$ : Fractional coordinates and lattice parameters used for the theoretical calculations, within the  $\text{P6}_3\text{mc}$  space group (No. 186).

| $a = 5.7487(2) \text{ \AA}$ and $c = 9.8656(4) \text{ \AA}$ |      |                                      |
|-------------------------------------------------------------|------|--------------------------------------|
| Atom                                                        | Site | (x, y, z)                            |
| Ni1                                                         | 2b   | (1/3, 2/3, 0.0546(6))                |
| Ni2                                                         | 2b   | (1/3, 2/3, 0.6172(5))                |
| Mo                                                          | 6c   | (0.1461(2), 0.8539(10), 0.3530(2))   |
| O <sub>1</sub>                                              | 2a   | (0, 0, 0.00000)                      |
| O <sub>2</sub>                                              | 2b   | (1/3, 2/3, 0.2552(2))                |
| O <sub>3</sub>                                              | 6c   | (0.4891(12), 0.5109(12), 0.4737(17)) |
| O <sub>4</sub>                                              | 6c   | (0.8317(12), 0.1683(12), 0.2422(18)) |

### Details of the DFT + eDMFT calculations

Tables S2-S6 summarize the fractionalized coordinates and lattice parameters used in this work. In DFT + eDMFT we used the nominal double-counting, which was shown in Ref. [S20] to be very close to the exact double-counting. The nominal double-counting uses the formula  $U(n_0 - 1/2) - J/2(n_0 - 1)$  with  $n_0$  for Mn, Fe, Co and Ni atoms of 5, 6, 7 and 8  $d$  electrons, respectively. We also checked that exact double-counting leads to very

TABLE S3.  $\text{Co}_2\text{Mo}_3\text{O}_8$ : Fractional coordinates and lattice parameters [S18] used for the theoretical calculations, within the  $P6_3mc$  space group (No. 186).

| $a = 5.76900 \text{ \AA}$ and $c = 9.90700 \text{ \AA}$ |      |                             |
|---------------------------------------------------------|------|-----------------------------|
| Atom                                                    | Site | (x, y, z)                   |
| Co1                                                     | 2b   | (1/3, 2/3, 0.05766)         |
| Co2                                                     | 2b   | (1/3, 2/3, 0.62158)         |
| Mo                                                      | 6c   | (0.14602, 0.85398, 0.35870) |
| O <sub>1</sub>                                          | 2a   | (0, 0, 0.00000)             |
| O <sub>2</sub>                                          | 2b   | (1/3, 2/3, 0.25420)         |
| O <sub>3</sub>                                          | 6c   | (0.48790, 0.51210, 0.47470) |
| O <sub>4</sub>                                          | 6c   | (0.83240, 0.16760, 0.24270) |

TABLE S4.  $\text{Fe}_2\text{Mo}_3\text{O}_8$ : Fractional coordinates and lattice parameters [S1] used for the theoretical calculations, within the  $P6_3mc$  space group (No. 186). The same crystal structure was used for the calculations of the  $\text{FeZnMo}_3\text{O}_8$  electronic properties, where Zn is situated on the distorted tetrahedral site.

| $a = 5.77530 \text{ \AA}$ and $c = 10.05880 \text{ \AA}$ |      |                             |
|----------------------------------------------------------|------|-----------------------------|
| Atom                                                     | Site | (x, y, z)                   |
| Fe1                                                      | 2b   | (1/3, 2/3, 0.06229)         |
| Fe2                                                      | 2b   | (1/3, 2/3, 0.62262)         |
| Mo                                                       | 6c   | (0.14605, 0.85395, 0.36029) |
| O <sub>1</sub>                                           | 2a   | (0, 0, 0.00000)             |
| O <sub>2</sub>                                           | 2b   | (1/3, 2/3, 0.25842)         |
| O <sub>3</sub>                                           | 6c   | (0.48694, 0.51306, 0.47226) |
| O <sub>4</sub>                                           | 6c   | (0.83375, 0.16625, 0.24630) |

similar solution with only minor differences in the details of the spectra. The robustness of the nominal double-counting allowed us to converge DTF + eDMFT solutions with charge converged criteria of  $10^{-5}$ , which is due to the statistical noise of the Monte Carlo impurity solver. We ensured that the details of the Kondo peak in the Fe  $e(1)$  orbitals are well

TABLE S5.  $\text{Mn}_2\text{Mo}_3\text{O}_8$ : Fractional coordinates and lattice parameters [S1] used for our theoretical calculations within the  $P6_3mc$  space group (No. 186).

| $a = 5.79750 \text{ \AA}$ and $c = 10.27070 \text{ \AA}$ |      |                             |
|----------------------------------------------------------|------|-----------------------------|
| Atom                                                     | Site | (x, y, z)                   |
| Mn1                                                      | 2b   | (1/3, 2/3, 0.06590)         |
| Mn2                                                      | 2b   | (1/3, 2/3, 0.62770)         |
| Mo                                                       | 6c   | (0.14591, 0.85409, 0.36469) |
| O <sub>1</sub>                                           | 2a   | (0, 0, 0.00000)             |
| O <sub>2</sub>                                           | 2b   | (1/3, 2/3, 0.26490)         |
| O <sub>3</sub>                                           | 6c   | (0.48780, 0.51220, 0.47190) |
| O <sub>4</sub>                                           | 6c   | (0.83560, 0.16440, 0.24920) |

TABLE S6.  $\text{Zn}_2\text{Mo}_3\text{O}_8$ : Fractional coordinates and lattice parameters [S19] used for our theoretical calculations within the  $P6_3mc$  space group (No. 186).

| $a = 5.78200 \text{ \AA}$ and $c = 9.93400 \text{ \AA}$ |      |                             |
|---------------------------------------------------------|------|-----------------------------|
| Atom                                                    | Site | (x, y, z)                   |
| Zn1                                                     | 2b   | (1/3, 2/3, 0.05688)         |
| Zn2                                                     | 2b   | (1/3, 2/3, 0.62272)         |
| Mo                                                      | 6c   | (0.14601, 0.85398, 0.35843) |
| O <sub>1</sub>                                          | 2a   | (0, 0, 0.00000)             |
| O <sub>2</sub>                                          | 2b   | (1/3, 2/3, 0.25440)         |
| O <sub>3</sub>                                          | 6c   | (0.48822, 0.51182, 0.47381) |
| O <sub>4</sub>                                          | 6c   | (0.83333, 0.16667, 0.24200) |

converged so that high-quality analytic continuation is possible.

To prove that the sharp peak in the Fe  $e(1)$  orbital on distorted tetrahedral side is of many-body origin, we examine the temperature dependence of the spectra [Fig. S14] along with the effect of varying the strength of the Coulomb interaction and Hund's coupling [Figs. S17 and S18]. In addition, we give further insights into the physical processes by examining the temperature dependence of the valence histogram [Fig. S16], and the role of

screening on the local susceptibility of both tetrahedral and octahedral sites [Fig. S15]. With all these checks performed, we can confidently conclude that the sharp peak at the edge of the valence band has a many-body origin and many similarities with the Kondo peak in metals, although here it appears at the edge of the valence band in an insulator.

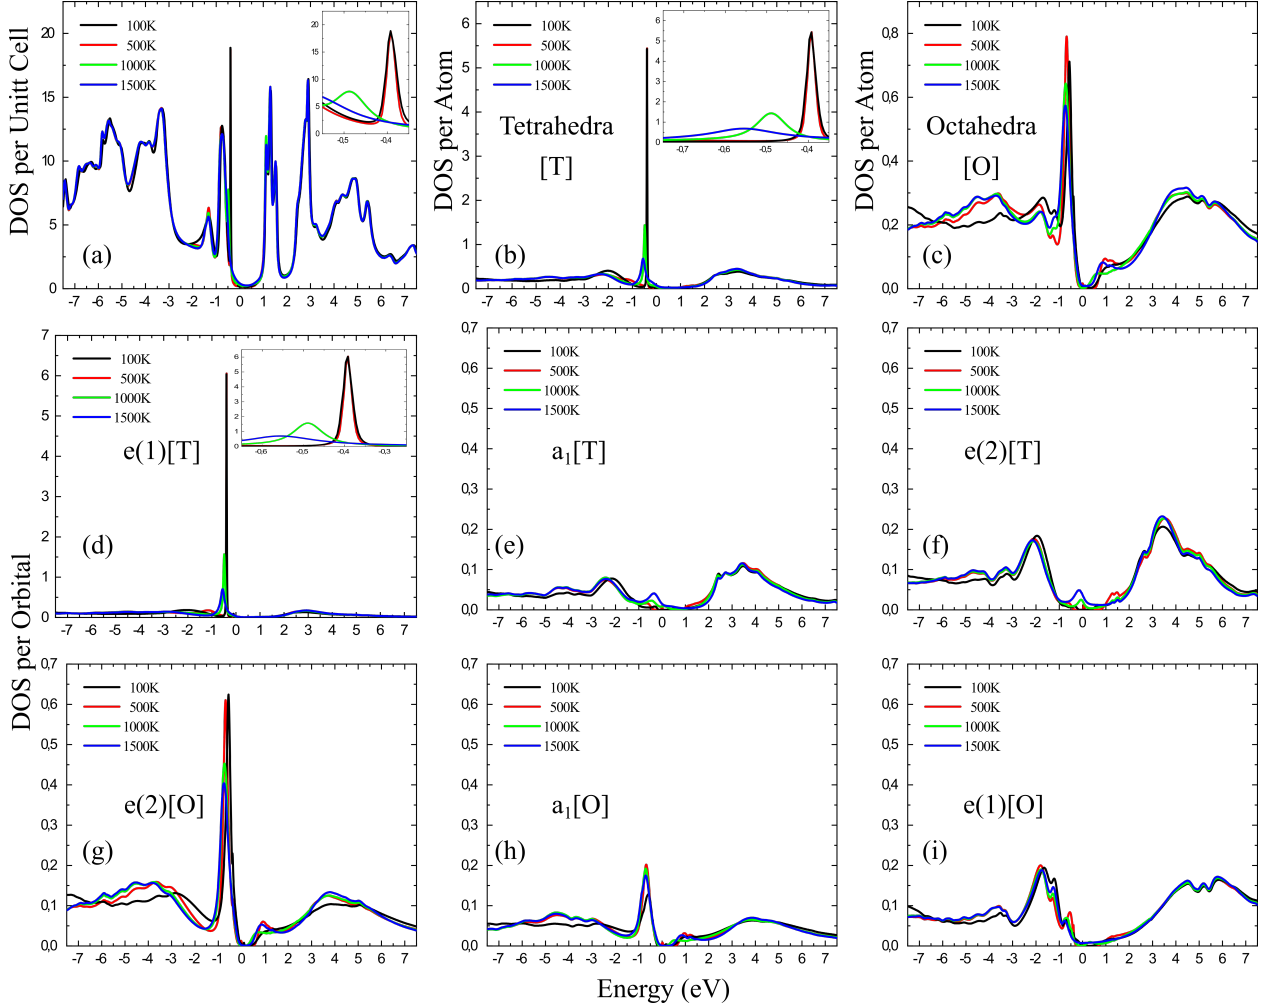

FIG. S14. Temperature dependent density of states (DOS) of  $\text{Fe}_2\text{Mo}_3\text{O}_8$ . Total DOS (a), and partial DOS on the Fe(T) (b) and Fe(O) (c) sites, respectively. Panels (d)-(i) display the orbitally-resolved partial density of states.

### Temperature dependence of the electronic structure

Figure S14 displays the temperature dependent density of states (DOS) of  $\text{Fe}_2\text{Mo}_3\text{O}_8$ . The sharp resonance at the top of the valence band is from the tetrahedral  $e(1)$  states, and the inset of panel (d) shows a close-up view of its temperature dependence. While the

peak is barely changed between 100 and 500 K, it is reduced by factor of three at 1000 K; it is nearly extinct at 1500 K. Its sudden collapse above 500 K is consistent with a many-body Kondo temperature of  $\approx 500$  K. The broader peak at the top of the valence band in panel (g), which originates from the  $e(2)$  orbital on distorted octahedral Fe site, also shows some temperature dependence, but its temperature variation is weak, and can be explained by normal temperature broadening of multiplet excitations, i.e., atomic-like excitations broadened by temperature smearing. The Kondo effect is, of course, usually studied in metals. Here we show that it can appear also in a complex insulator, which has both Mott- and band gaps. The orbital with the weak Mott-like gap can develop a many-body excitation near the edge of the band, which is used to screen magnetic moment - as in normal metallic Kondo effect. The emergence of this peak in  $\text{Fe}_2\text{Mo}_3\text{O}_8$  reduces the size of the optical gap and explains the unique optical spectrum of this compound.

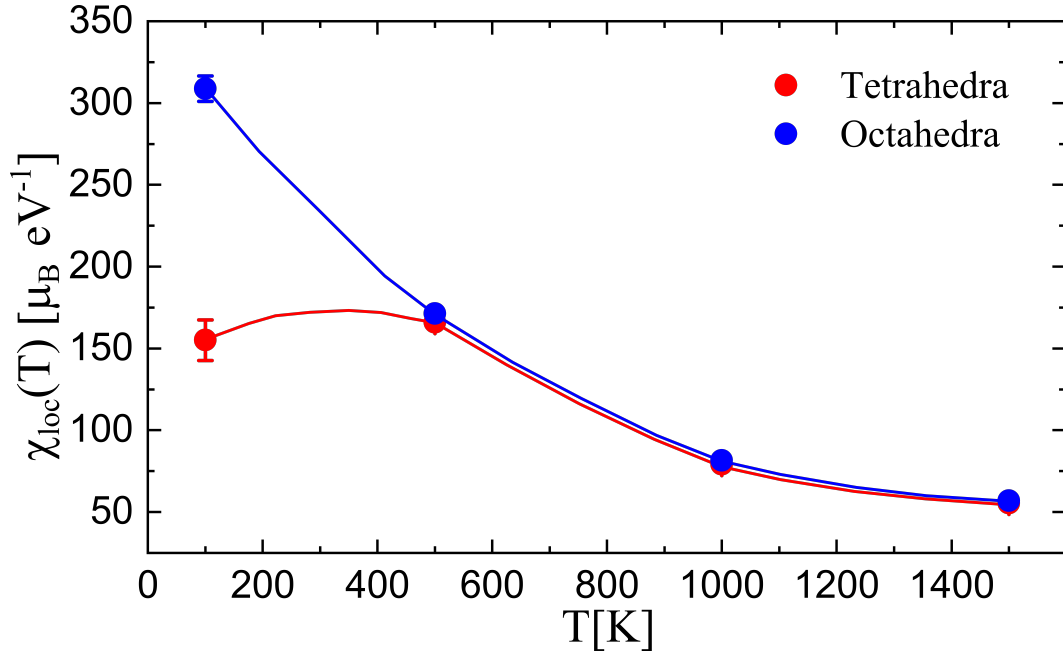

FIG. S15. Temperature dependence of the local susceptibility computed for the Fe(O) and Fe(T) sites in  $\text{Fe}_2\text{Mo}_3\text{O}_8$ . The tetrahedral site susceptibility saturates once the many-body peak in the spectral function is fully formed. The local susceptibility is defined as  $\chi_{loc} [\mu_B^2 \text{ eV}^{-1}] = \mu_{eff}^2 * \beta / 3$ , where  $\beta [\text{eV}^{-1}] = 11604 / T [\text{K}]$  and  $\mu_{eff}^2$  is  $g^2 S(S+1)$  in the atomic limit.

To verify that the peak in the spectral function has many-body character, we computed the local spin susceptibility at zero frequency on both the tetrahedral and octahedral iron

sites. At high temperature, both sites show identical Curie-Weiss temperature dependence. Below 500 K, the tetrahedral site shows saturated susceptibility, whereas the octahedral site still shows Curie-Weiss behavior. The saturated susceptibility on the tetrahedral site confirms that the fluctuating magnetic moment, which is present at high temperature, is arrested below 500 K, - the temperature at which the many-body resonance is fully formed.

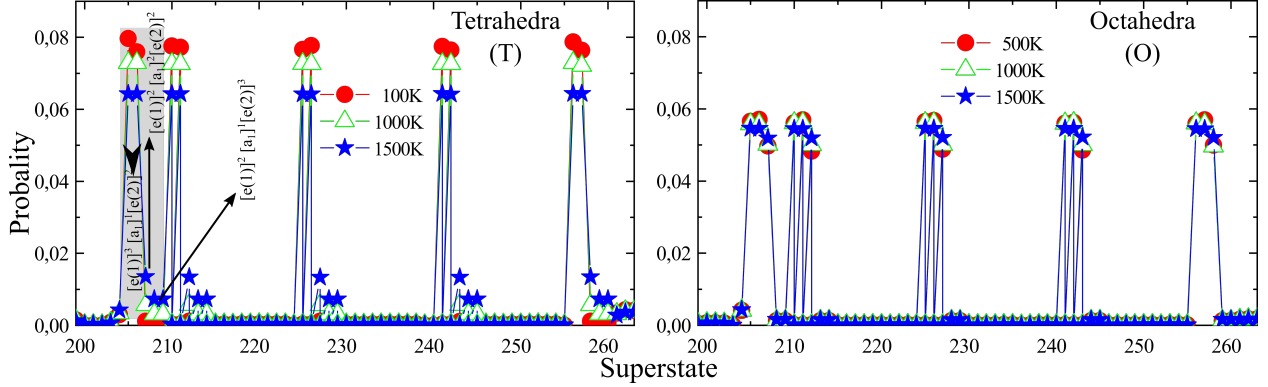

FIG. S16.  $\text{Fe}_2\text{Mo}_3\text{O}_8$ : Temperature dependent Probability of the atomic superstates for the Fe ions inside the distorted tetrahedra and octahedra. Various superstates correspond to the same occupation of the individual orbitals but with different spin orientation (up versus down), as shown in the left panel for the tetrahedra. For example, the  $[e(1)]^3$ ,  $[a_1]^1$  and  $[e(2)]^2$  notation corresponds to three electrons inside the  $e(1)$  orbital (two spin up and one spin down), one electron spin up in the  $a_1$  orbital and two electrons spin up in the  $e(2)$  orbital. The superstate numbers on the x-axis represent an internal label of the code and it runs from 0 to 1024 (the total number of superstates for the  $d$  shell). The gray area shows the independent orbital occupations that repeat themselves, for various spin configurations. For example, the states around labels 255-260 have the same electron occupation as the states in the gray area, but the electrons have opposite spins.

To gain further insight into the temperature dependence of the many-body state, we show the valence histogram summarizes the probability of atomic states in the thermal evolution Fig. S16. There are 1024 atomic states for each  $d$ -orbital on an Fe atom, and we select those that have the highest probability for this plot. On the tetrahedral site, the highest probability is for the state pictorially drawn in Fig. 4 of the main text. Three electrons are on the  $e(1)$  whereas the  $a_1$  and  $e(2)$  orbitals host a single electron in a high spin state. This state has 5-fold degeneracy. Hence, the cumulative probability for this atomic ground state is around 80%. The tetrahedral site shows substantially more temperature dependence

than the octahedral site. We see that with increasing temperature, the  $e(1)$  orbital loses some of the electrons, so that the sixth electron (the single electron beyond half-filled high spin state) is distributed more uniformly among the  $e(1)$ ,  $a_1$ , and  $e(2)$  states, achieving larger degeneracy and larger entropy. The  $e(1)$ , therefore achieves higher spin, which is less efficiently screened at elevated temperature.

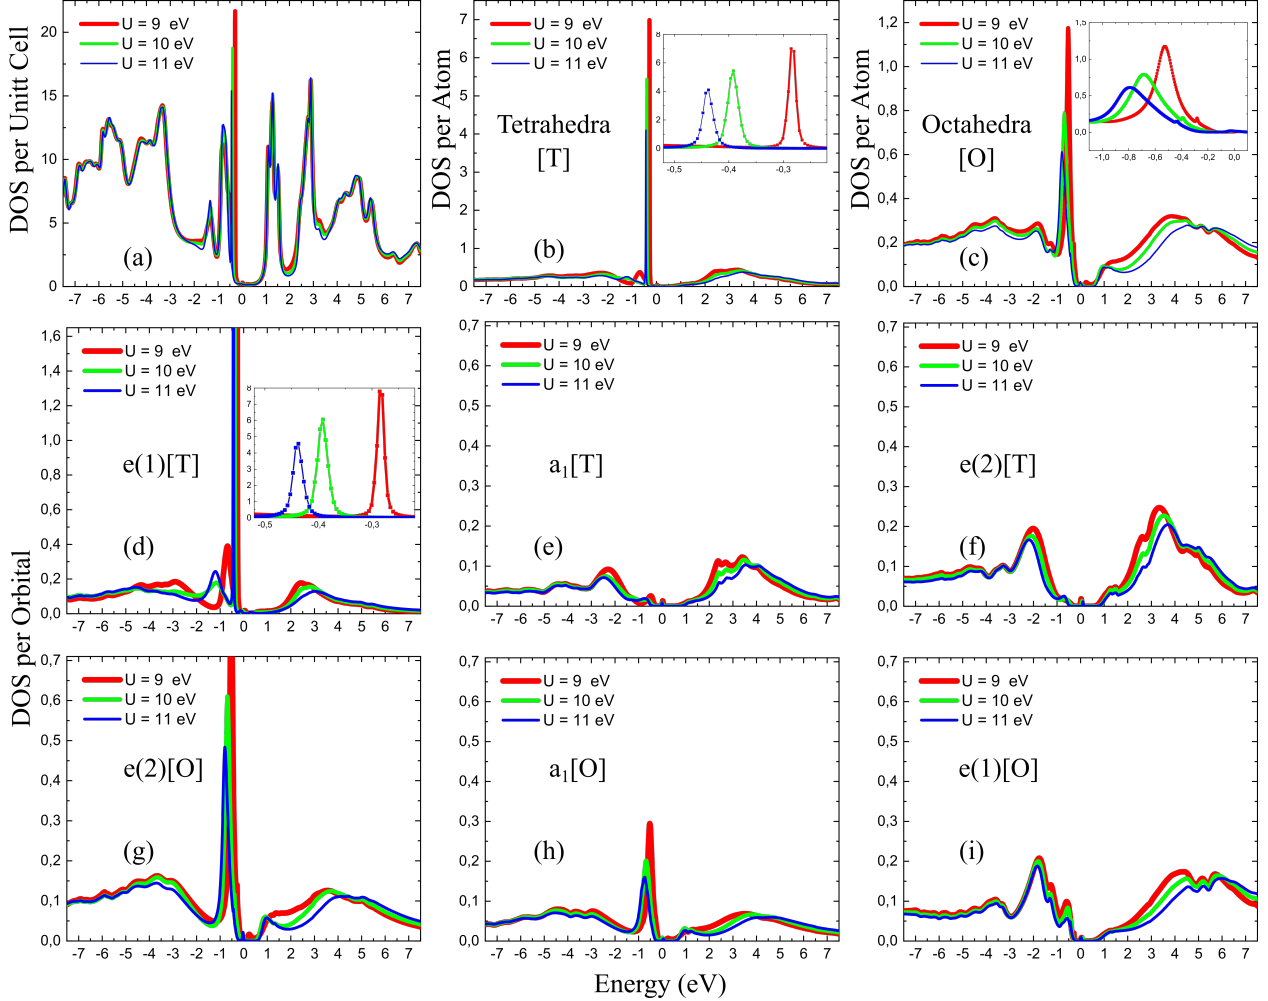

FIG. S17.  $\text{Fe}_2\text{Mo}_3\text{O}_8$ :  $U$ -dependent density of states.

### Coulomb repulsion strength

Finally, we tested how the many-body resonance depends upon the strength of the Coulomb repulsion. As a reminder, atomic-like excitations are expected to be shifted proportionally to the change in the screened Coulomb repulsion (or change in Hund's coupling). The broad band excitations are expected to shift by a similar amount as the chemical potential

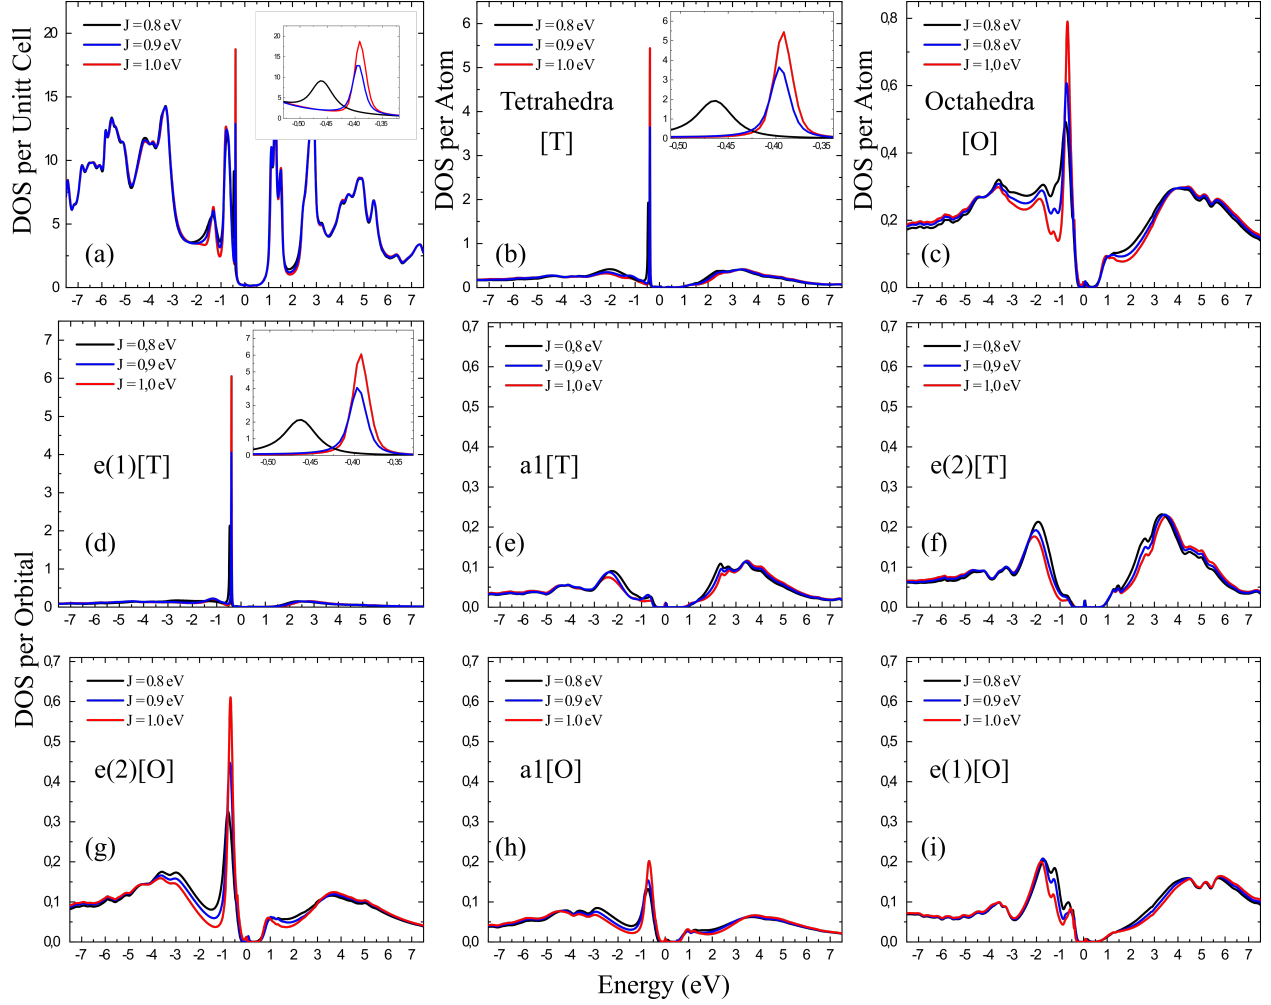

FIG. S18.  $\text{Fe}_2\text{Mo}_3\text{O}_8$ :  $J$ -dependent density of states.

is adjusted. On the other hand, the Kondo peak strength and in particular the Kondo temperature scale is expected to be most sensitive to the strength of the Coulomb repulsion. Our estimated value of  $U$  and  $J$  in this class of materials is 10 and 1.0 eV, respectively.

Figures S17 and S18 show how the DOS depends upon  $U$  and  $J$ , respectively. As is clear from both figures, the sharp resonance on the distorted octahedral site is somewhat reduced with increasing  $U$ , whereas it is slightly enhanced with increasing Hund's coupling  $J$ . The  $U$  dependence can be explained by the fact that the Kondo temperature is reduced by increasing  $U$ . In the most simple version of the symmetric single-impurity Anderson impurity problem, the Kondo temperature has the form  $T_k \propto \exp(-U/\Delta)$ , where  $\Delta$  is a number related to the strength of the hybridization. Of course we do not expect this relation to hold in this material, nevertheless the reduction of  $T_k$  with increasing  $U$  is expected, which reduces the

strength of the Kondo peak at room temperature.

The sharpening of the resonance with increasing Hund's coupling is related to the fact that the half-filled  $N = 5$  high spin state of maximal spin  $5/2$  shifts closer to the ground state of  $N = 6$  configuration (spin  $S = 2$ ) with increasing  $J$ . Hence, we are effectively reducing the impurity bound-state energy  $E_d$ , which has similar effect on the Kondo temperature  $T_k$  as the Coulomb repulsion  $U$ . In the extremely asymmetric Anderson model, where  $U$  is very large, the Kondo temperature has the form  $T_k \propto \exp(-|E_d|/\Delta)$ , where  $E_d$  is the energy difference between the ground and excited state with different charge. As the increased Hund's coupling reduces effective  $E_d$ , we expect the resonance to grow.

Overall, the presence of the sharp resonance at the edge of the valence band is a robust feature of DFT+eDMFT solution for  $\text{Fe}_2\text{Mo}_3\text{O}_8$ , even though the strength and sharpness of the peak, as well as its temperature dependence changes somewhat with the choice of Coulomb repulsion parameters.

### Simulating the impact of hybridization

It is well known that the many-body Kondo resonance can exist only if the hybridization function at the peak is finite, and that the Kondo scale is exponentially sensitive to the value of the hybridization at that frequency. The hybridization function is encoding the screening processes, which couple the local degrees of freedom with the itinerant carriers in the system. Moreover, it is well known that in the Hubbard-like models, the Kondo-like peak develops simultaneously in the local spectral function as well as in the hybridization function, enhancing the screening with reducing the temperature. The same occurs in  $\text{Fe}_2\text{Mo}_3\text{O}_8$ , except that the resonance does not appear at the Fermi level, but rather at the top of the valence band in the insulator.

To prove that this sharp resonance has Kondo-like origin, we removed the sharp resonance from the hybridization function, and observe its impact on the local spectral function. If the resonance is atomic like in nature, i.e., a multiplet state, the peak will not be affected by the small change in the hybridization function. On the other hand, if the peak is Kondo-like, the small change in the hybridization function will have a profound effect on the spectral function. In Fig. S19(a) we show the Fe density of states when hybridization function is self-consistently determined (hybridization-ON) and when we cut out a small portion of the

hybridization in the window around the peak ( $-0.44\text{eV}$  to  $-0.17\text{eV}$ ), denoted by hybridization-OFF. As can be seen in the figure, the peak disappears at that energy (of  $-0.4\text{eV}$ ), and a smaller and broader peak appears at lower energy ( $-0.58\text{eV}$ ) where the hybridization function is still finite. The same resonance is visible in Mo-d states as well as O-p states, proving that the sharp peak is a mixture of the local degrees of freedom on the iron ( Fe spin), as well as the itinerant states on Mo and O, which screen the iron spin.

In Fig. S20 we show the effect of increasing temperature, which also has similar effect of reducing screening. The fact that the temperature has such a profound effect on the peak strength, as well as the fact that the value of the hybridization at the peaks energy is essential for its development, is a proof that the sharp peak is many body in nature.

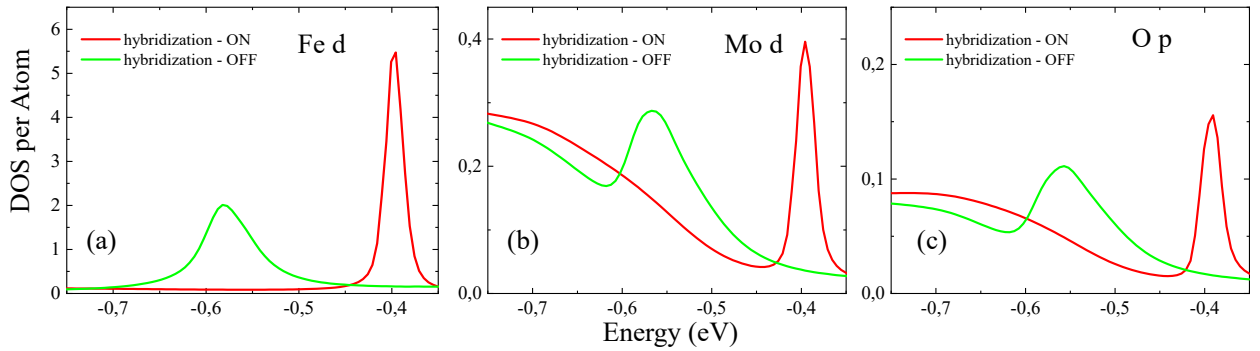

FIG. S19. Atom projected density of states for  $\text{Fe}_2\text{Mo}_3\text{O}_8$ , computed using the self-consistent hybridization (red curve labelled “hybridization-ON”) and the manually reduced hybridization in the energy region of the Kondo-like peak (green curve labelled “hybridization-OFF”), as explained in the text. Panels (a), (b) and (c) show the atom projected density of states for Fe  $d$ , Mo  $d$ , and one of the inequivalent O  $p$  atoms in the unit cell.

## Magnetic calculations

It can be seen in Fig. S21, that the Kondo peak found at the top of the valence band in the  $e(1)$  orbital, almost disappears in the ordered state.

---

[S1] T. N. Stanislavchuk, G. L. Pascut, A. P. Litvinchuk, Z. Liu, S. Choi, M. J. Gutmann, B. Gao, K. Haule, V. Kiryukhin, S.-W. Cheong, and A. A. Sirenko, *Spectroscopic and first principle*

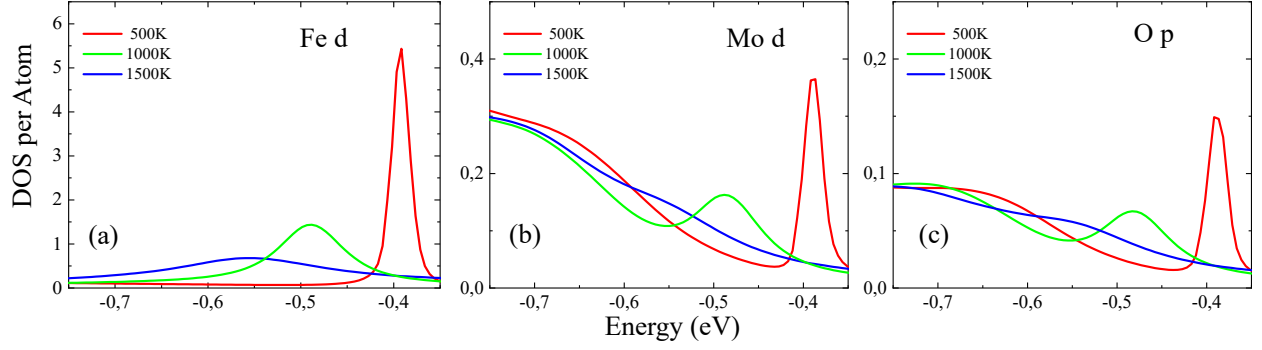

FIG. S20. Temperature dependent atom projected density of states for  $\text{Fe}_2\text{Mo}_3\text{O}_8$ . Panels (a), (b) and (c) show the atom projected density of states for Fe  $d$ , Mo  $d$ , and one of the inequivalent O  $p$  atoms in the unit cell.

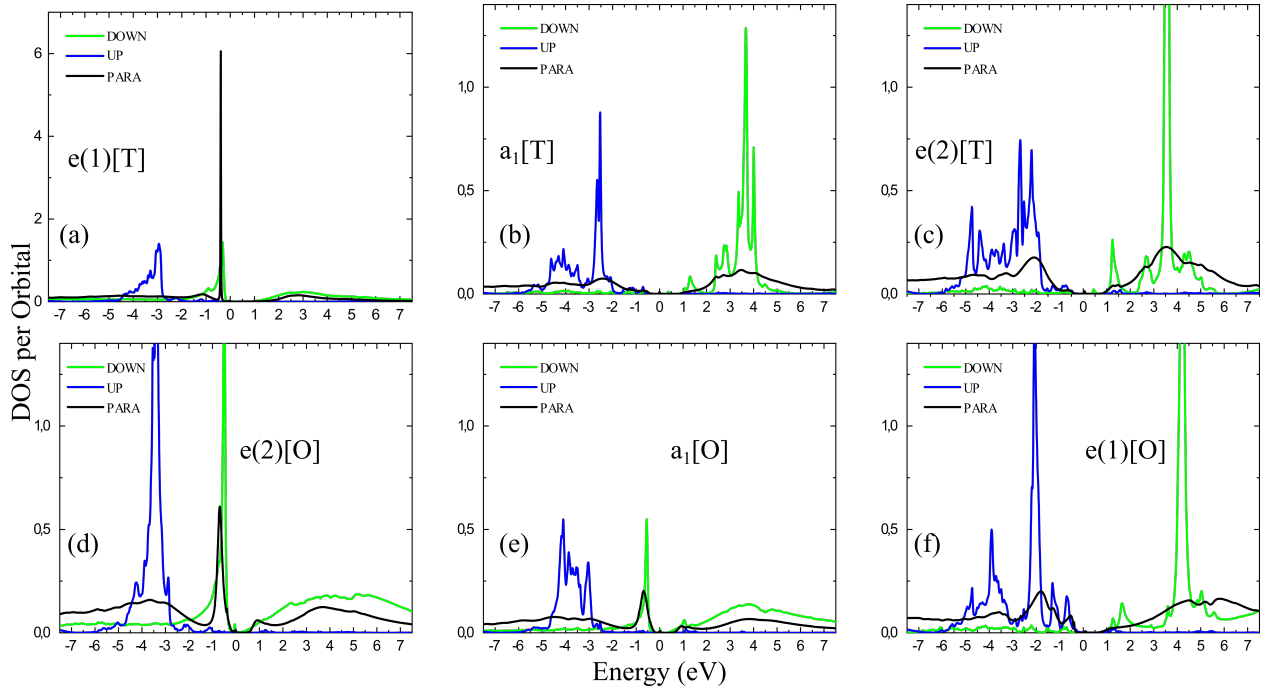

FIG. S21.  $\text{Fe}_2\text{Mo}_3\text{O}_8$ : Magnetic versus paramagnetic orbital- and spin-projected density of states.

*DFT+eDMFT study of complex structural, electronic, and vibrational properties of  $M_2\text{Mo}_3\text{O}_8$  ( $M = \text{Fe}, \text{Mn}$ ) polar magnets*, Phys. Rev. B **102**, 115139 (2020).

[S2] S. Reschke, A. A. Tsirlin, N. Khan, L. Prodan, V. Tsurkan, I. Kézsmárki, and J. Deisenhofer, *Structure, phonons, and orbital degrees of freedom in  $\text{Fe}_2\text{Mo}_3\text{O}_8$* , Phys. Rev. B **102**, 094307 (2020).

[S3] P. K. Sarswat and M. L. Free, *A study of energy band gap versus temperature for  $\text{Cu}_2\text{ZnSnS}_4$  thin films*, Physica B: Condensed Matter **407**, 108 (2012).

- [S4] K. P. O'Donnell and X. Chen, *Temperature dependence of semiconductor band gaps*, Applied Physics Letters **58**, 2924 (1991).
- [S5]  $\text{Fe}_2\text{Mo}_3\text{O}_8$  ( $\text{Mo}_3\text{Fe}_2\text{O}_8$ ) Crystal Structure: Datasheet from “PAULING FILE Multinaries Edition – 2012” in SpringerMaterials ([https://materials.springer.com/isp/crystallographic/docs/sd\\_2041523](https://materials.springer.com/isp/crystallographic/docs/sd_2041523)), Copyright 2016 Springer-Verlag Berlin Heidelberg & Material Phases Data System (MPDS), Switzerland & National Institute for Materials Science (NIMS), Japan.
- [S6] K. R. O'Neal, A. Al-Wahish, Z. Li, P. Chen, J. W. Kim, S.-W. Cheong, G. Dhallenne, A. Revcolevschi, X.-T. Chen, and J. L. Musfeldt, *Vibronic coupling and band gap trends in  $\text{CuGeO}_3$  nanorods*, Physical Review B **96**, 075437 (2017).
- [S7] K. R. O'Neal, A. Paul, A. Al-Wahish, K. D. Hughey, A. L. Blockmon, X. Luo, S.-W. Cheong, V. S. Zapf, C. V. Topping, J. Singleton, M. Ozerov, T. Birol, and J. L. Musfeldt, *Spin-lattice and electron-phonon coupling in 3d/5d hybrid  $\text{Sr}_3\text{NiIrO}_6$* , npj Quantum Materials **4**, 48 (2019).
- [S8] C.J. Ballhausen, *Introduction to Ligand Field Theory*, McGraw-Hill (1962).
- [S9] A.M. Stoneham, *Theory of Defects in Solids: Electronic Structure of Defects in Insulators and Semiconductors*, Clarendon Press (2001).
- [S10] J. W. Evans, T. R. Harris, B. R. Reddy, K. L. Schepler, and P. A. Berry, *Optical spectroscopy and modeling of  $\text{Fe}^{2+}$  ions in zinc selenide*, Journal of Luminescence **188**, 541 (2017).
- [S11] Y. Wang, G. L. Pascut, B. Gao, T. A. Tyson, K. Haule, V. Kiryukhin, and S.-W. Cheong, *Unveiling hidden ferrimagnetism and giant magnetoelectricity in polar magnet  $\text{Fe}_2\text{Mo}_3\text{O}_8$* , Scientific Reports **5**, 12268 (2015).
- [S12] Oxford Diffraction Ltd., *Version 1.171.36.21*, CrysAlisPro **release 14-08-2012 CrysAlis171.NET** (2010).
- [S13] V. Petříček, M. Dušek, and L. Palatinus, *Crystallographic Computing System JANA2006: General features*, Zeitschrift für Kristallographie - Crystalline Materials **229** (2014), 10.1515/zkri-2014-1737.
- [S14] R. C. Clark and J. S. Reid, *The analytical calculation of absorption in multifaceted crystals*, Acta Crystallographica Section A Foundations of Crystallography **51**, 887 (1995).
- [S15] P. J. Becker and P. Coppens, *Extinction within the limit of validity of the Darwin transfer equations. I. General formalism for primary and secondary extinction and their applications*

- to spherical crystals*, Acta Crystallographica Section A **30**, 129 (1974).
- [S16] K. Momma and F. Izumi, *VESTA 3 for three-dimensional visualization of crystal, volumetric and morphology data*, Journal of Applied Crystallography **44**, 1272 (2011).
- [S17] Inkscape.org, Draw Freely — Inkscape (2020).
- [S18] H. Abe, A. Sato, N. Tsujii, T. Furubayashi, and M. Shimoda, *Structural refinement of  $T_2Mo_3O_8$  ( $T=Mg, Co, Zn$  and  $Mn$ ) and anomalous valence of trinuclear molybdenum clusters in  $Mn_2Mo_3O_8$* , Journal of Solid State Chemistry **183**, 379 (2010).
- [S19] J. Cuny, P. Gougeon, and P. Gall, *Redetermination of  $Zn_2Mo_3O_8$* , Acta Crystallographica Section E Structure Reports Online **65**, i51 (2009).
- [S20] K. Haule, *Exact Double Counting in Combining the Dynamical Mean Field Theory and the Density Functional Theory*, Phys. Rev. Lett. **115**, 196403 (2015).
- [S21] K. Haule, *DFT + Embedded DMFT Functional*, <http://hauleweb.rutgers.edu/tutorials/>.
